# Supplementary material for: Collective eXplainable AI: Explaining Cooperative Strategies and Agent Contribution in Multiagent Reinforcement Learning with Shapley Values
Source: arXiv:2110.01307 source file (2021-10-04)
Supplement: Supplementary file 1 [file appendix.tex]

\section*{Additional results}
% The following tables detail the hyperparameters used for the experiments described in Section \ref{sec:experiments}.
We conducted extra experiments attempting to test the scalability of models in Experiment 2 (see Subsection \ref{subsec:exp_speeds}) by increasing the number of agents to 9 predators and 3 preys. However,
running over 500,000 episodes MADDPG did not
make the predators global reward converge. When observing the model, contrary to the one used in Experiment 1 (see Subsection \ref{subsec:exp_1}) agents do not show any collective cooperative strategy and wander aimlessly on the map failing to catch the prey (except when randomly hitting them). We hypothesize that the high number of agents makes cooperation between them difficult and this may be pointed out as a limitation of MADDPG.

We also tried to use Value-Decomposition Networks (VDN) \cite{sunehag2017valuedecomposition} to train a model for the Harvest \cite{SSDOpenSource} environment but this was not successful since the model struggled to converge and did not converged to a positive mean reward while A3C reached around 500 of mean reward, see Fig. \ref{fig:harvest_learning_curve}).

\begin{figure}[H]
    \centering
    \includegraphics[width=\linewidth]{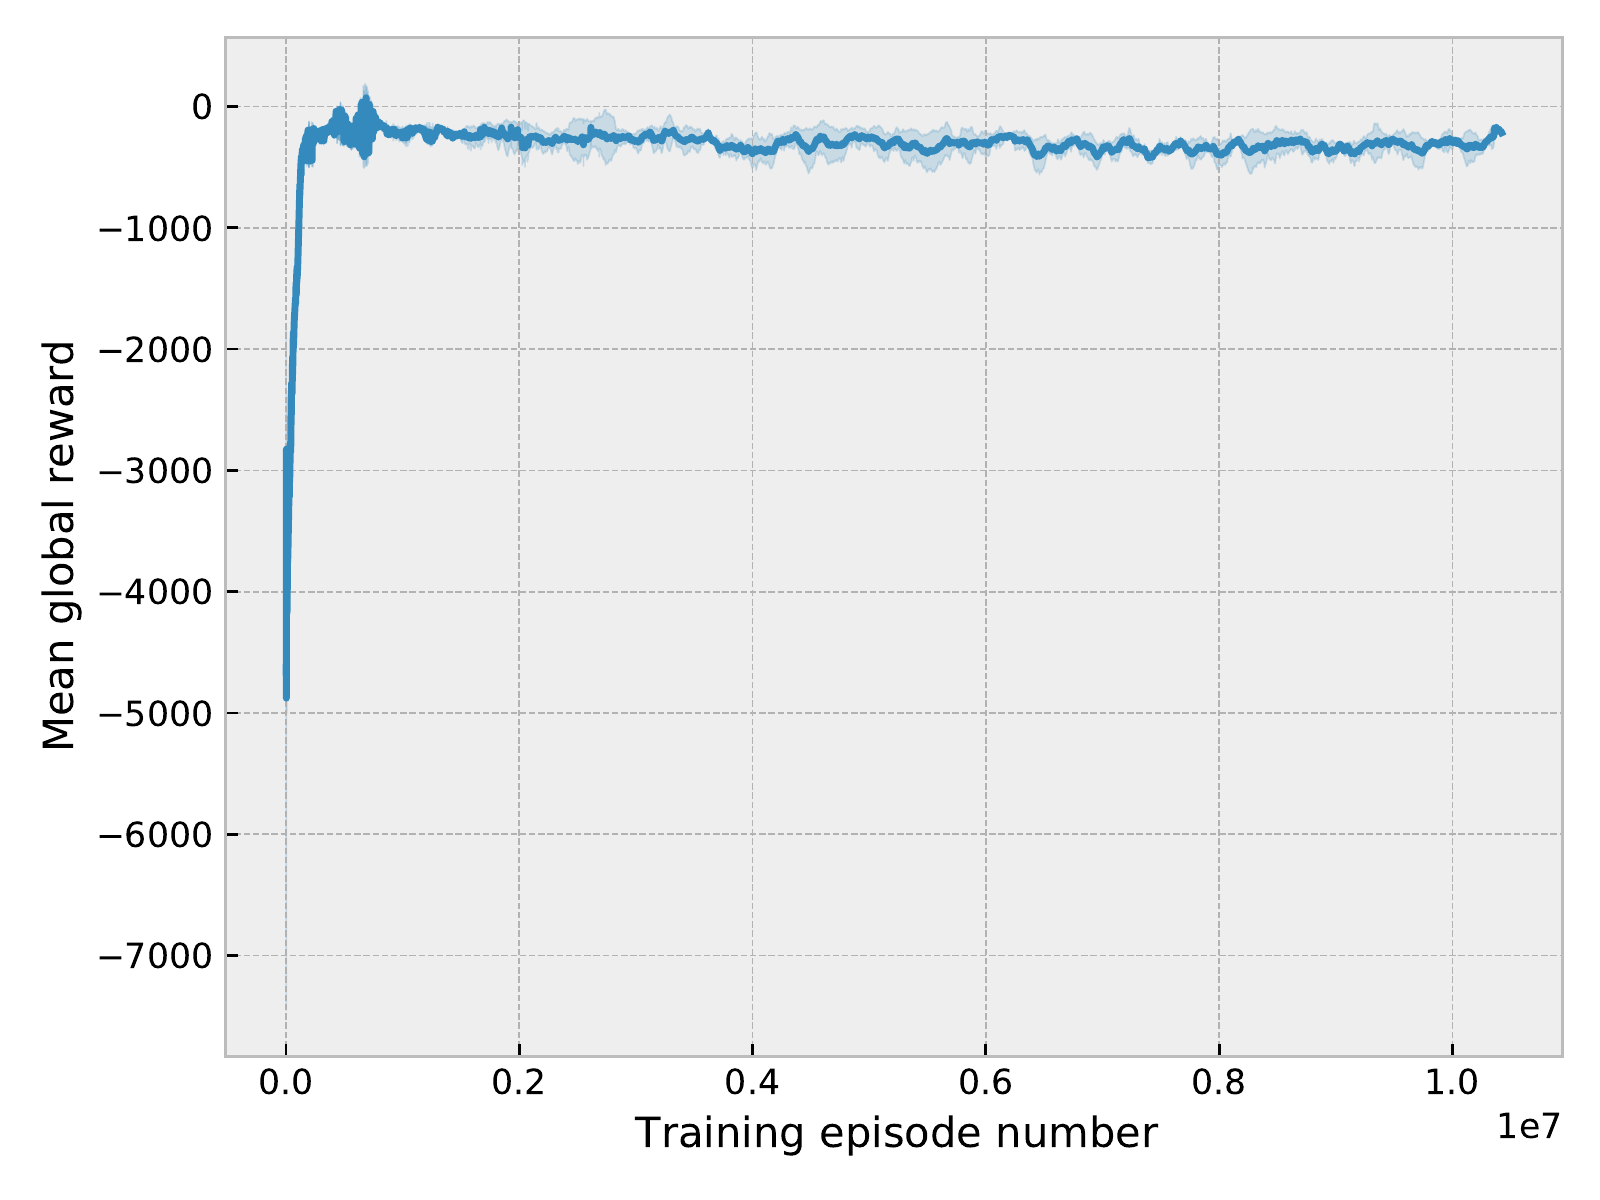}
    \caption{Learning curve of the Harvest VDN model (averaged over 3 runs). We can clearly see that the model did not reach a way lower max reward than the A3C model in Fig. \ref{fig:harvest_learning_curve}}
    \label{fig:qmix_lc}
\end{figure}

\section*{Social Metrics Per Agent}

We further studied the social metrics presented in Subsection \ref{subsec:harvest_social} and introduced in \cite{perolat2017multiagent}. We refactored them into a per agent basis in order to make a more relevant comparison with Shapley values. Considering agent $i$ among $N$ agents, we obtained the following formulas:

\begin{equation}
    U_i = \mathbb{E}\left[\frac{R_i}{T}\right]
    \label{eq:efficency_per_agent}
\end{equation}
\begin{equation}
    S_i = t_i = \mathbb{E}[t/r^{i}_{t}>0]
\end{equation}
\begin{equation}
    E_i = 1 - \frac{\sum_{j=1}^{N}|R_i-R_j|}{2\sum_{j=1}^{N}R_j}
\end{equation}
Where $R_i$ is the reward obtained by agent $i$.
Using these refactored formulas, we plotted the metrics using the same data than in Subsection \ref{subsec:harvest_social} in Fig. \ref{fig:efficiency_per_agent}, Fig. \ref{fig:sustainability_per_agent} and Fig. \ref{fig:equality_per_agent}.
\begin{figure}[!ht]
    \centering
    \includegraphics[width=\linewidth]{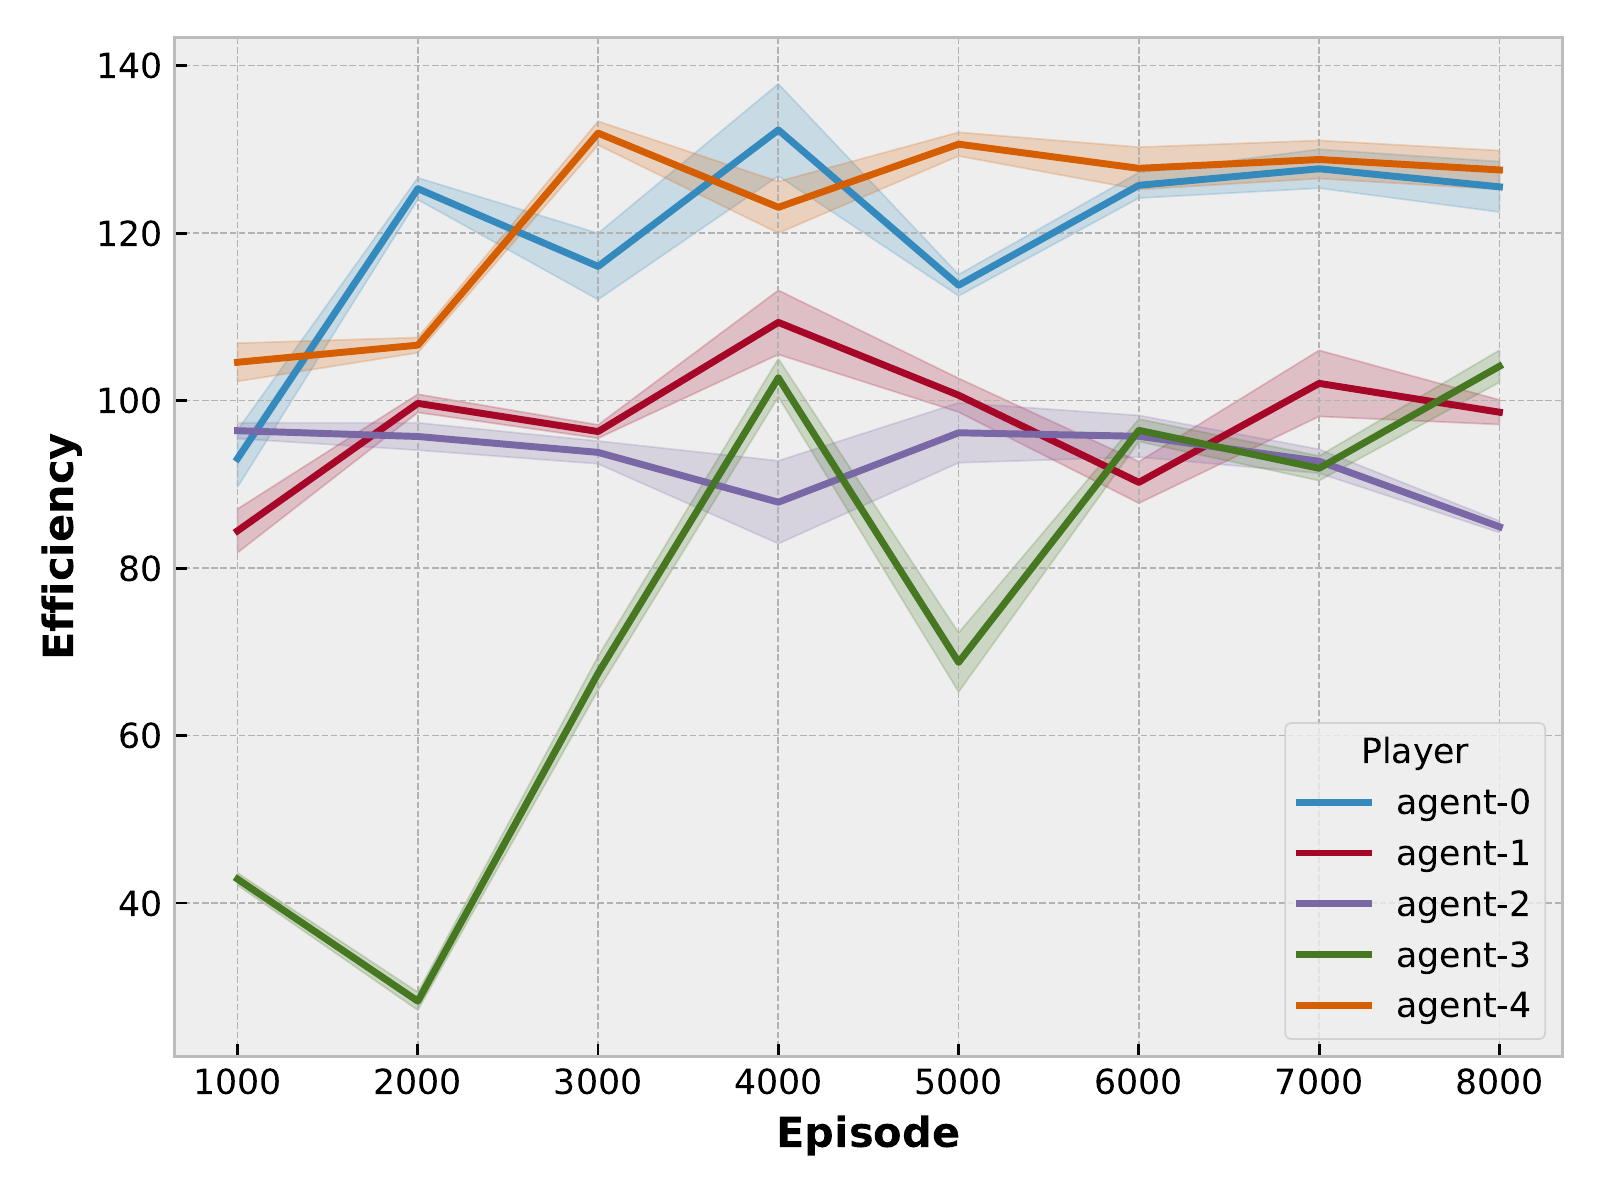}
    \caption{Evolution of \textit{Efficiency} social metric per agent over several episodes (averaged on 4 runs).}
    \label{fig:efficiency_per_agent}
\end{figure}

\begin{figure}[H]
    \centering
    \includegraphics[width=\linewidth]{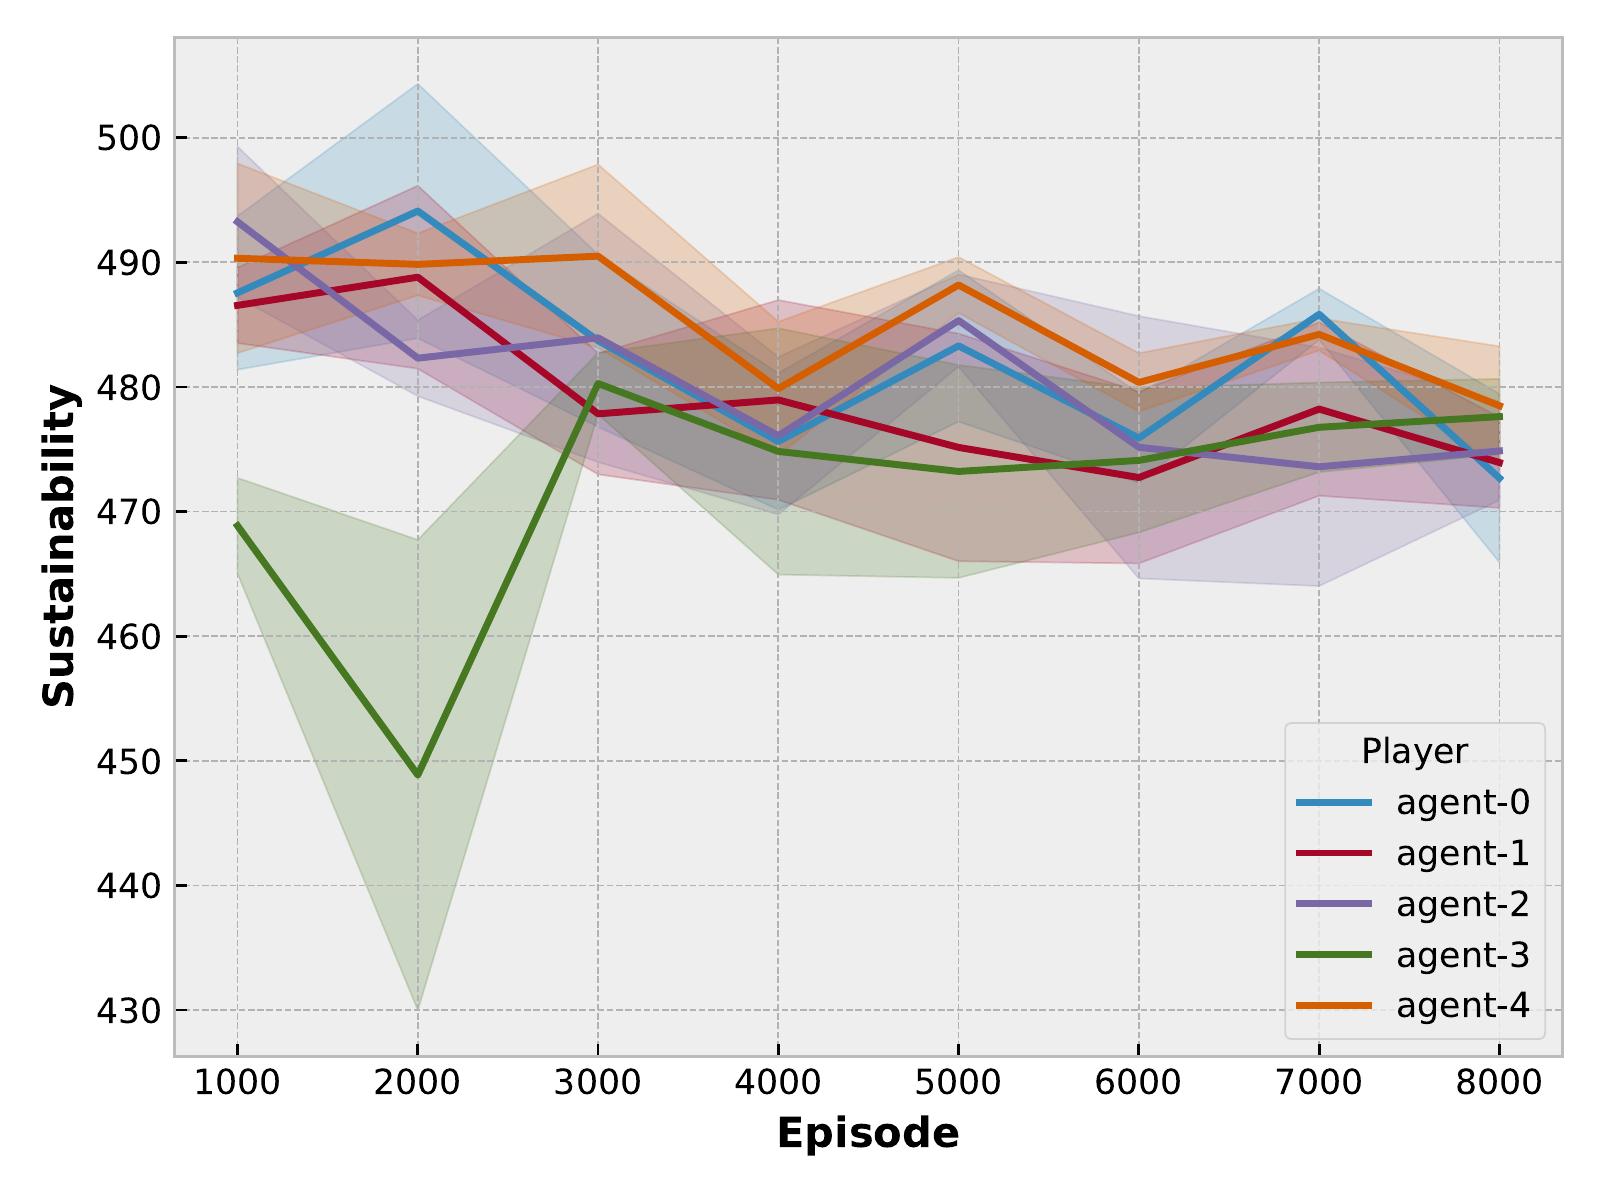}
    \caption{Evolution of Sustainability per agent over several episodes (averaged on 4 runs).}
    \label{fig:sustainability_per_agent}
\end{figure}

\begin{figure}[H]
    \centering
    \includegraphics[width=\linewidth]{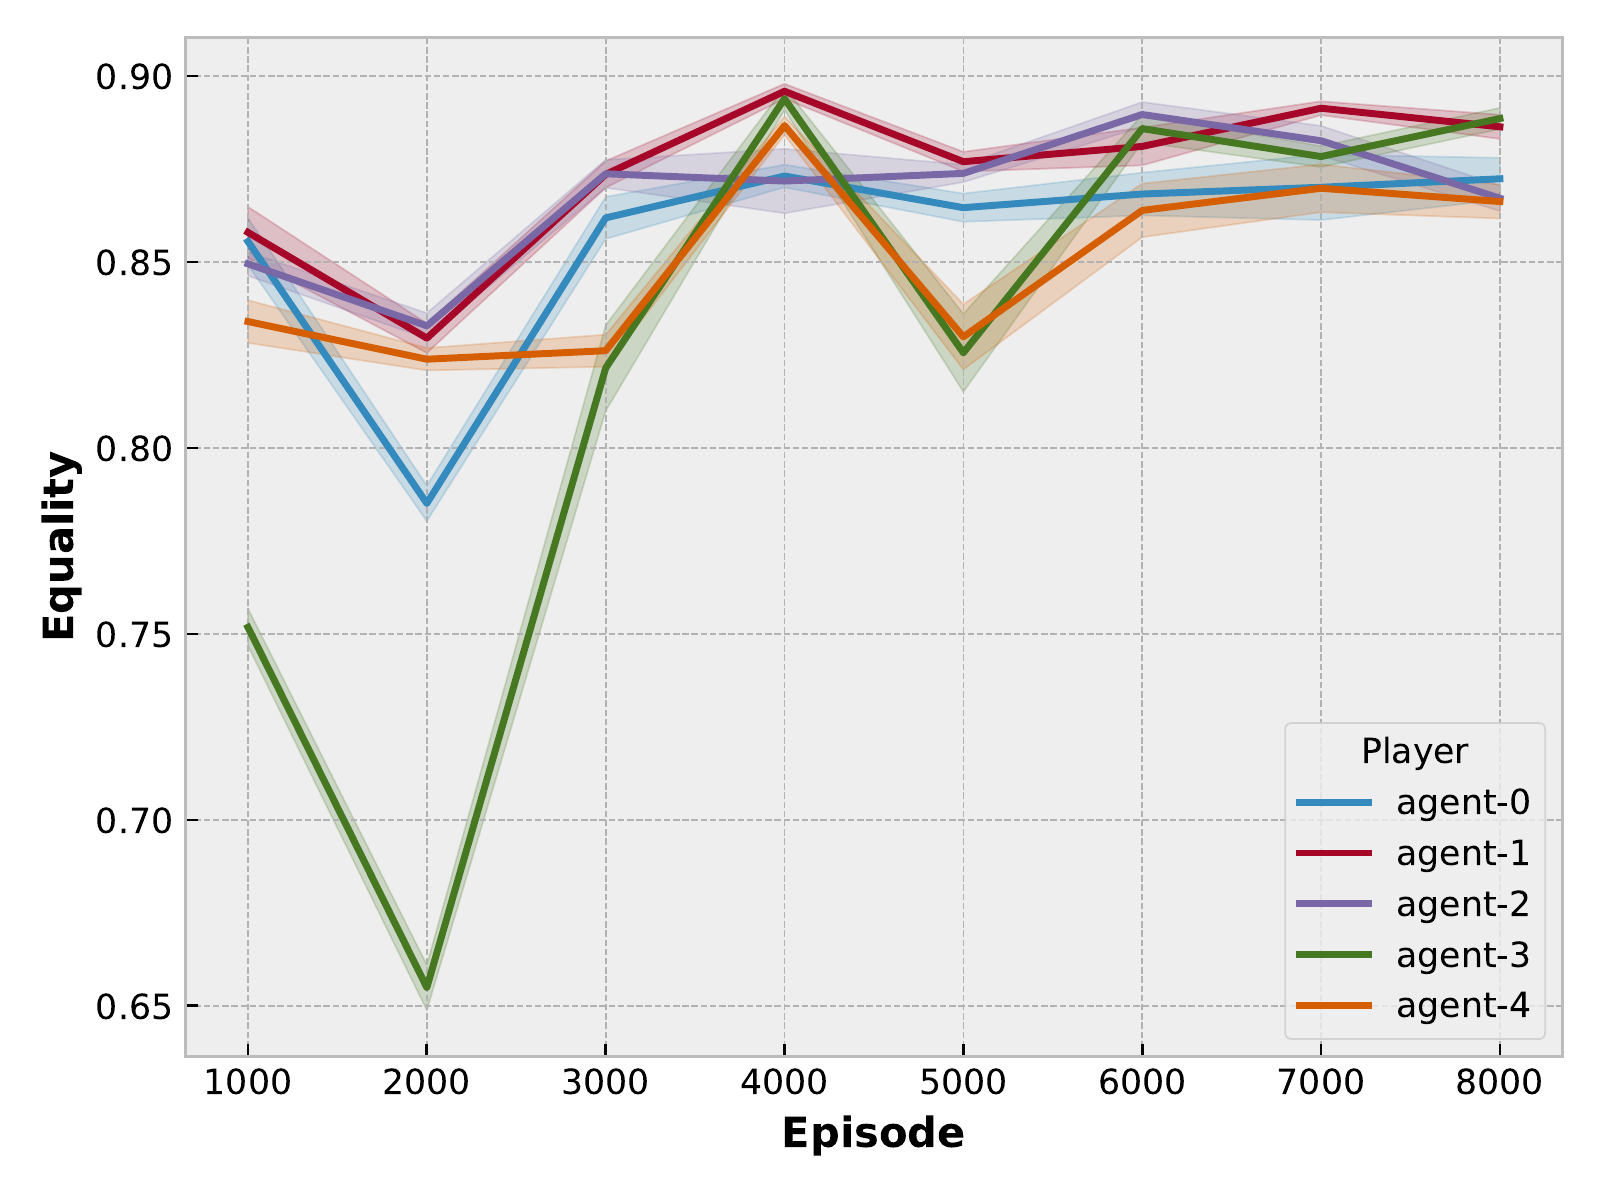}
    \caption{Evolution of Equality per agent over several episodes (averaged on 4 runs).}
    \label{fig:equality_per_agent}
\end{figure}

When analyzing these figures, we can clearly see that Efficiency (Fig. \ref{fig:efficiency_per_agent}) is identical to the plot of Shapley values (Fig. \ref{fig:social_metrics_harvest}). That is a logical result since the efficiency per agent (Eq. \ref{eq:efficency_per_agent}) computes the same result than Shapley values: the average contribution (reward) per agent. Equality (Fig. \ref{fig:equality_per_agent}) also follows the same trend as Shapley values. This visual correlation supports our claim that Shapley values is a relevant tool to assert the contribution of agents in RL cooperative settings.

\section*{Experimental Details}

Here we present some additional details about the setup of the experiments showcased in Section \ref{sec:experiments}.

 \begin{table}[H]%tbp!]
    \centering
    \begin{tabular}{cc}
        \toprule
        \textbf{Parameter} &  \textbf{Value} \\
        \midrule
          Learning Rate &  0.01 \\
          Optimizer & Adam \\
          Number of MLP units & 128 \\
          Discount Factor & 0.95 \\
          Batch Size & 1024 \\
        \bottomrule
    \end{tabular}
    \caption{Hyperparameters used for every MADDPG and DDPG model on Predator-Prey scenario. These are the default parameters recommended by \cite{lowe2017multi}. Other hyperparameters (e.g., the number of predators or their speed) may vary and their values are indicated in the experimental settings description (Subsections \ref{subsec:exp1_settings} and \ref{subsec:exp2_settings}).}
    \label{tab:pp_hparams}
\end{table}

 \begin{table}[H]%tbp!]
     \centering
     \begin{tabular}{cc}
        \toprule
          \textbf{Parameter} &  \textbf{Value} \\
          \midrule
          Learning Rate &  0.0001 \\
          Optimizer & Adam \\
          Number of MLP units & 128 \\
          Discount Factor & 0.99 \\
          Batch Size & 30000 \\
        \bottomrule
    \end{tabular}
    \caption{Hyperparameters used for A3C models on Harvest scenario. These are the default parameters recommended by \cite{SSDOpenSource}. Other hyperparameters (e.g. the number of agents) may vary and their values are indicated in the experimental settings description (see Subsection \ref{subsec:exp4_settings}).}
    \label{tab:harvest_hparams}
 \end{table}

% ADD LEARNING CURVES

\begin{figure}[H]
    \centering
    \includegraphics[width=\linewidth]{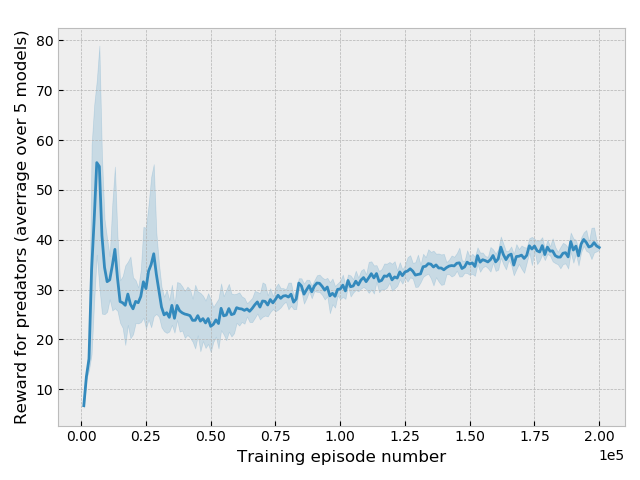}
    \caption{Learning curve of the Prey-Predator MADDPG models (average over 5 models) used in Experiment 1.}
    \label{fig:prey_predator_lc}
\end{figure}

\begin{figure}[H]
    \centering
    \includegraphics[width=\linewidth]{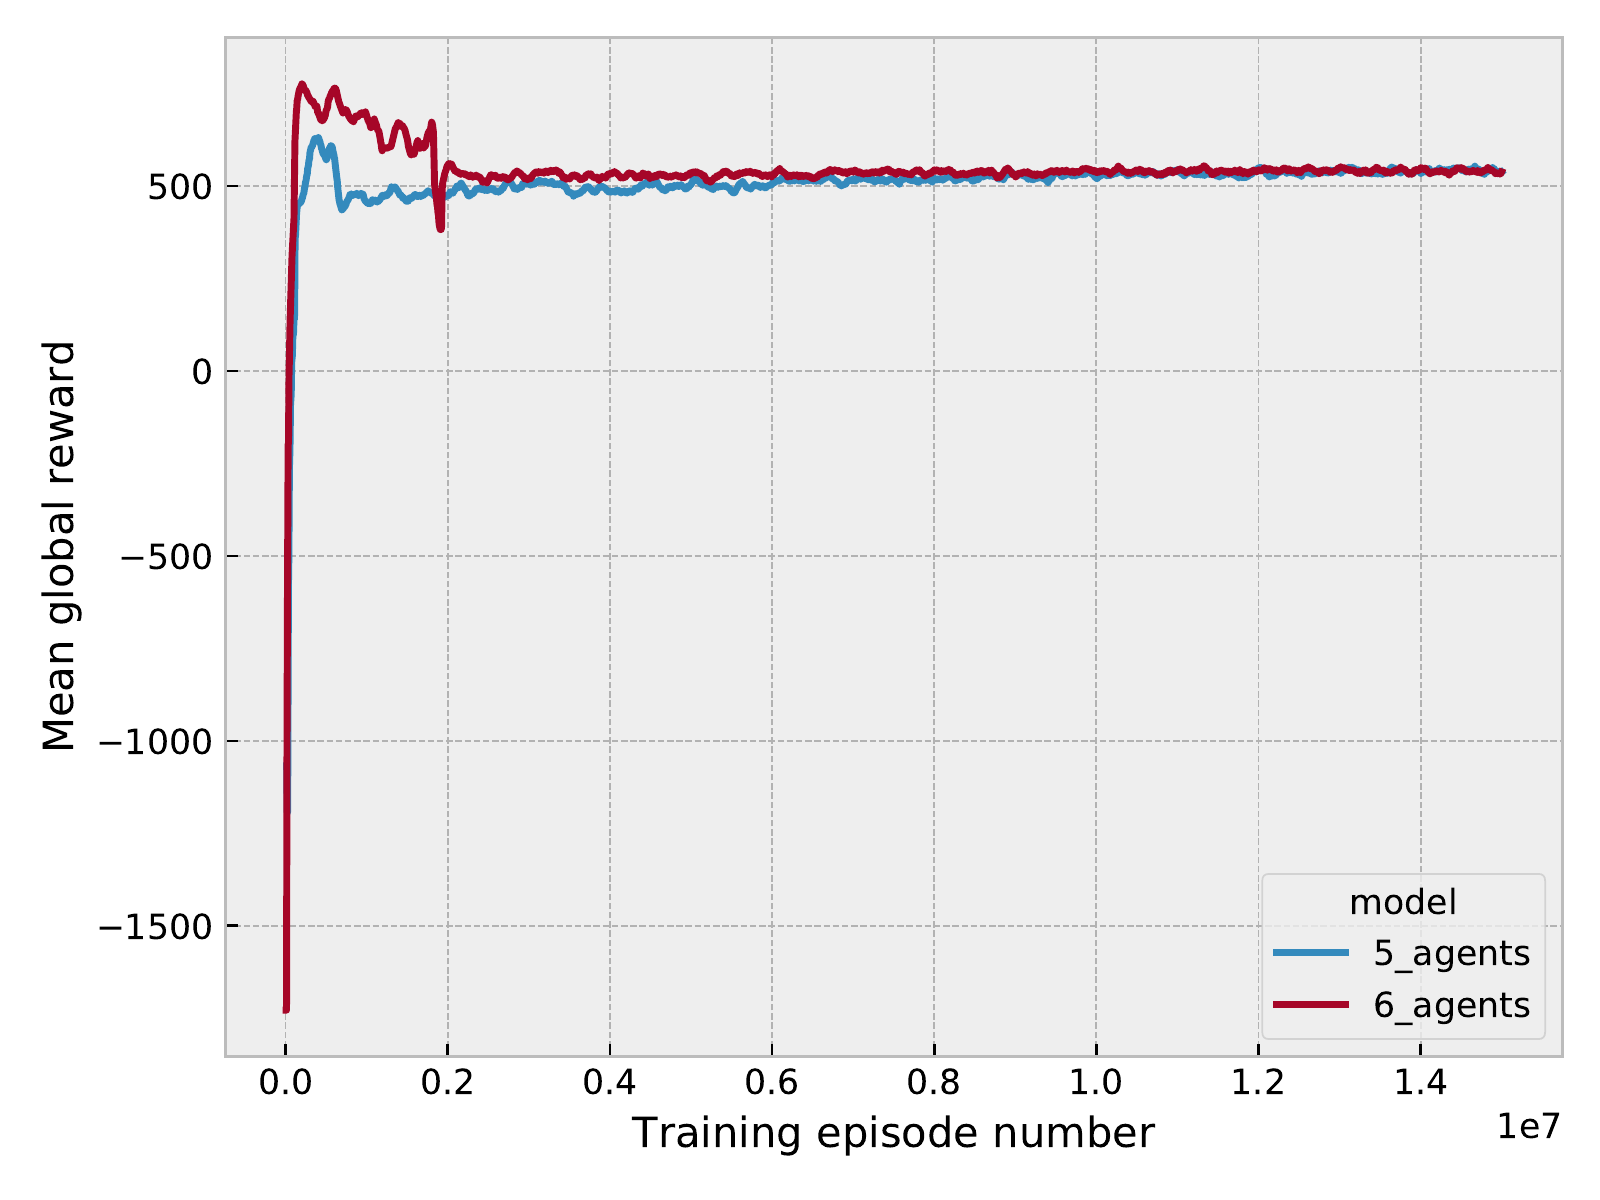}
    \caption{Learning curve of the Harvest A3C models (5 and 6 agents models used in Experiment 3). We can clearly observe that both models quickly converge to the same reward.}
    \label{fig:harvest_learning_curve} 
\end{figure}
